# Supplementary material for: Density Functional Theory of Model Systems with the Biaxial Nematic Phase
Source: arXiv:0907.1044 source file (2009-07-03)
Supplement: Supplementary file 2 [file appendix_smectic.tex]

\chapter{Bifurcations to smectic phases}
\label{ap:smecticbif}
 Here we present the bifurcation equations when the smectic phase
is taken into account. As we have mentioned, if we neglect the spatially
non-uniform state as a reference, we have five extra bifurcation scenarios,
those are: nematic biaxial -- smectic biaxial,
nematic uniaxial -- smectic uniaxial, nematic uniaxial -- smectic biaxial,
isotropic -- smectic biaxial, isotropic -- smectic uniaxial. We list the
formulas for these transitions. For clarity we have dropped the average 
symbols, i.e. $S_{l,m,n}\equiv\average{S_{l,m,n}}$.
\nl 1) nematic uniaxial -- smectic uniaxial:
\begin{equation}
\begin{split}
 S_{0,0,0} = & \, \frac{1}{2} \rho \lsbra w_s S_{0,0,0}+ w_{0,0} S_{2,0,0} \Delta _{2,0,0}+ w_{2,2} S_{2,0,2} \Delta _{2,0,2}+w_{0,2} \left( S_{2,0,2} \Delta _{2,0,0}+ S_{2,0,0} \Delta_{2,0,2}\right) \rsbra \, , \\
 S_{2,0,0} = & \, \frac{1}{70} \rho  A_0 w_{0,0} S_{2,0,0}+\frac{1}{70} \rho  B_0 w_{2,2} S_{2,0,2}+\frac{1}{70} \rho  w_{0,2} \left(B_0 S_{2,0,0}+A_0 S_{2,0,2}\right)+\frac{1}{2} \rho  w_s S_{0,0,0} \Delta _{2,0,0} \, , \\
 S_{2,0,2} = & \, \frac{1}{70} \rho  B_2 w_{0,0} S_{2,0,0}+\frac{1}{70} \text{C} \rho  w_{2,2} S_{2,0,2}+\frac{1}{70} \rho  w_{0,2} \left(\text{C} S_{2,0,0}+B_2 S_{2,0,2}\right)+\frac{1}{2} \rho  w_s S_{0,0,0} \Delta _{2,0,2} \, ,
\end{split}
\end{equation}
where
\begin{equation}
\begin{split}
 A_{0} = & \, 7+10 \Delta _{2,0,0}+18 \Delta _{4,0,0}=A_{2} \, , \\
 B_{0} = & \, -10 \Delta _{2,0,2}+3 \sqrt{15} \Delta _{4,0,2}=B_{2} \, \\
 C_{0} = & \, 7-10 \Delta _{2,0,0}+3 \Delta _{4,0,0}+3 \sqrt{35} \Delta _{4,0,4} \, .
\end{split}
\end{equation}
\nl 2) nematic uniaxial -- smectic biaxial:
\begin{equation}
\begin{split}
 S_{2,2,0} = & \, \frac{1}{70} \rho  A_0 w_{0,0} S_{2,2,0}+\frac{1}{140} \rho  B_0 w_{2,2} S_{2,2,2}+\frac{1}{140} \rho  w_{0,2} \left(B_0 S_{2,2,0}+2 A_0 S_{2,2,2}\right) \, , \\
 S_{2,2,2} = & \, \frac{1}{140} \rho  A_2 w_{0,0} S_{2,2,0}+\frac{1}{140} \rho  B_2 w_{2,2} S_{2,2,2}+\frac{1}{140} \rho  w_{0,2} \left(B_2 S_{2,2,0}+A_2 S_{2,2,2}\right) \, ,
\end{split}
\end{equation}
where
\begin{equation}
\begin{split}
 A_{0} = & \, 7-10 \Delta _{2,0,0}+3 \Delta _{4,0,0} \, \\
 B_{0} = & \, 20 \Delta _{2,0,2}+\sqrt{15} \Delta _{4,0,2}=A_{2} \, . \\
 B_{2} = & \, 14+20 \Delta _{2,0,0}+\Delta _{4,0,0}+\sqrt{35} \Delta _{4,0,4} \, .
\end{split}
\end{equation}
\nl 3) nematic biaxial -- smectic biaxial:
\begin{equation}
\begin{split}
 S_{0,0,0} = & \, \frac{1}{2} \rho  \left(w_s S_{0,0,0}+w_{0,0} \left(S_{2,0,0} \Delta _{2,0,0}+S_{2,2,0} \Delta _{2,2,0}\right)+\right.\\
 & w_{0,2} \left(S_{2,0,2} \Delta _{2,0,0}+S_{2,0,0} \Delta _{2,0,2}+S_{2,2,2} \Delta _{2,2,0}+S_{2,2,0} \Delta _{2,2,2}\right)+\\
 & \left.w_{2,2} \left(S_{2,0,2} \Delta _{2,0,2}+S_{2,2,2} \Delta _{2,2,2}\right)\right) \, , \\
 S_{2,0,0} = & \, \frac{1}{70} \rho  w_{0,0} \left(A_{200} S_{2,0,0}+C_{200} S_{2,2,0}\right)+\\
 & \frac{1}{140} \rho  w_{0,2} \left(2 B_{200} S_{2,0,0}+2 A_{200} S_{2,0,2}+5 D_{200} S_{2,2,0}+2 C_{200} S_{2,2,2}\right)+\\
 & \frac{1}{140} \rho  w_{2,2} \left(2 B_{200} S_{2,0,2}+5 D_{200} S_{2,2,2}\right)+\frac{1}{2} \rho  w_s S_{0,0,0} \Delta _{2,0,0} \, , \\
 S_{2,0,2} = & \, \frac{1}{140} \rho  w_{0,0} \left(2 A_{202} S_{2,0,0}+5 B_{202} S_{2,2,0}\right)+\\
 & \frac{1}{140} \rho  w_{0,2} \left(D_{202} S_{2,0,0}+2 A_{202} S_{2,0,2}+C_{202} S_{2,2,0}+5 B_{202} S_{2,2,2}\right)+\\
 & \frac{1}{140} \rho  w_{2,2} \left(D_{202} S_{2,0,2}+C_{202} S_{2,2,2}\right)+\frac{1}{2} \rho  w_s S_{0,0,0} \Delta _{2,0,2} \, , \\
 S_{2,2,0} = & \, \frac{1}{70} \rho  w_{0,0} \left(A_{220} S_{2,0,0}+\left(7+B_{220}\right) S_{2,2,0}\right)+\\
 & \frac{1}{140} \rho  w_{0,2} \left(5 D_{220} S_{2,0,0}+2 A_{220} S_{2,0,2}+C_{220} S_{2,2,0}+2 \left(7+B_{220}\right) S_{2,2,2}\right)+\\
 & \frac{1}{140} \rho  w_{2,2} \left(5 D_{220} S_{2,0,2}+C_{220} S_{2,2,2}\right)+\frac{1}{2} \rho  w_s S_{0,0,0} \Delta _{2,2,0} \, , \\
 S_{2,2,2} = & \, \frac{1}{140} \rho  w_{0,0} \left(5 D_{222} S_{2,0,0}+C_{222} S_{2,2,0}\right)+\frac{1}{140} \rho  w_{2,2} \left(B_{222} S_{2,0,2}+A_{222}
 S_{2,2,2}\right)+\\
 & \frac{1}{140} \rho  w_{0,2} \left(B_{222} S_{2,0,0}+5 D_{222} S_{2,0,2}+A_{222} S_{2,2,0}+C_{222} S_{2,2,2}\right)+\frac{1}{2} \rho  w_s S_{0,0,0} \Delta _{2,2,2} \, .
\end{split}
\end{equation}
where
\begin{equation}
\begin{split}
 A_{200} = & \, 7+10 \Delta _{2,0,0}+18 \Delta _{4,0,0} \, , \\
 B_{200} = & \, -10 \Delta _{2,0,2}+3 \sqrt{15} \Delta _{4,0,2} \, , \\
 C_{200} = & \, -10 \Delta _{2,2,0}+3 \sqrt{15} \Delta _{4,2,0} \, , \\
 D_{200} = & \, D_{202}=D_{220}=D_{222}=4 \Delta _{2,2,2}+3 \Delta _{4,2,2} \, , \\
 A_{202} = & \, -10 \Delta _{2,0,2}+3 \sqrt{15} \Delta _{4,0,2} \, , \\
 B_{202} = & \, 14-20 \Delta _{2,0,0}+6 \Delta _{4,0,0}+6 \sqrt{35} \Delta _{4,0,4} \, , \\
 C_{202} = & \, B_{222} = 20 \Delta _{2,2,0}+\sqrt{15} \Delta _{4,2,0}+5 \sqrt{21} \Delta _{4,2,4} \, , \\
 A_{220} = & \, -10 \Delta _{2,2,0}+3 \sqrt{15} \Delta _{4,2,0} \, , \\
 B_{220} = & \, -10 \Delta _{2,0,0}+3 \Delta _{4,0,0}+3 \sqrt{35} \Delta _{4,4,0} \, , \\
 C_{220} = & \, C_{222}=20 \Delta _{2,0,2}+\sqrt{15} \Delta _{4,0,2}+5 \sqrt{21} \Delta _{4,4,2} \, , \\
 A_{222} = & \, 14+20 \Delta _{2,0,0}+\Delta _{4,0,0}+\sqrt{35} \Delta _{4,0,4}+\sqrt{35} \Delta _{4,4,0}+35 \Delta _{4,4,4} \, , \\
\end{split}
\end{equation}
4,5) isotropic-smectic biaxial transition:
\begin{equation}
\begin{split}
 & \left(-2+\rho  w_s\right) S_{0,0,0}=0 \, , \\
 & \left(-10+\rho  w_{0,0}\right) S_{2,0,0}+\rho  w_{0,2} S_{2,0,2}=0 \, , \\
 & \rho  w_{0,2} S_{2,0,0}+\left(-10+\rho  w_{2,2}\right) S_{2,0,2}=0 \, , \\
 & \left(-10+\rho  w_{0,0}\right) S_{2,2,0}+\rho  w_{0,2} S_{2,2,2}=0 \, , \\
 & \rho  w_{0,2} S_{2,2,0}+\left(-10+\rho  w_{2,2}\right) S_{2,2,2}=0 \, .
\end{split}
\end{equation}
