# Supplementary material for: Density Functional Theory of Model Systems with the Biaxial Nematic Phase
Source: arXiv:0907.1044 source file (2009-07-03)
Supplement: Supplementary file 6 [file appendix_nextorder.tex]

\chapter{Next order corrections}
\label{ap:nextorder}
 It is of some interest to present the next order corrections,
as well as for angular momentum $L$ higher than $2$, as for density expansion.
We show those in here.
